# Supplementary material for: Deep Random Splines for Point Process Intensity Estimation of Neural Population Data
Source: arXiv:1903.02610 ancillary file (2019-12-29)
Supplement: Supplementary file 1 [file drs_appendix.pdf]

# Appendix for "Deep Random Splines for Point Process Intensity Estimation of Neural Population Data"

## Appendix 1: Parameterization for nonnegative splines of even degree

As mentioned on section 2.1, there is an alternative characterization of nonnegative polynomials of even degree $d = 2k$ on an interval $[l, u)$ that is analogous to equation 1 of the manuscript, which says that the polynomial $p$ is nonnegative on the interval if and only if it can be written as:

$$p(t) = [t]^\top Q_1[t] + (u - t)(t - l)\tilde{[t]}^\top Q_2\tilde{[t]}$$

where again, $[t] = (1, t, t^2, \ldots, t^k)^\top$ and $Q_1$ is a $(k + 1) \times (k + 1)$ symmetric positive semidefinite matrix. In this case $Q_2$ is now a $k \times k$ symmetric positive semidefinite matrix and $\tilde{[t]} = (1, t, t^2, \ldots, t^{k-1})^\top$. Again, it follows that a piecewise polynomial of degree $d$ with knots $t_0, \ldots, t_I$ defined as $p^{(i)}(t)$ for $t \in [t_{i-1}, t_i)$ for $i = 1, \ldots, I$ is nonnegative if and only if it can be written as:

$$p^{(i)}(t) = [t]^\top Q_1^{(i)}[t] + (t_i - t)(t - t_{i-1})\tilde{[t]}^\top Q_2^{(i)}\tilde{[t]}$$

for $i = 1, \ldots, I$, where each $Q_1^{(i)}$ is a $(k + 1) \times (k + 1)$ symmetric positive semidefinite matrix and each $Q_2^{(i)}$ is a $k \times k$ symmetric positive semidefinite matrix.

## Appendix 2: Projecting onto the space of smooth splines

As mentioned in section 2.2, mapping to $\Psi = \cap_{j=0}^{s+1}\mathcal{C}_j$ can be achieved through the method of alternating projections. As mentioned previously, projecting onto $\mathcal{C}_0$ can be easily done through eigen-decomposition. We now go through the details on how to project onto the other $\mathcal{C}_j$ sets. We will only cover $\mathcal{C}_1$, $\mathcal{C}_2$ and $\mathcal{C}_3$ for odd-degree splines as we used splines of degree 3 and smoothness 2, but projecting onto $\mathcal{C}_j$ for $j \geq 4$ for higher degree splines can be done in an analogous way. Projections for even degree splines can also be derived in an analogous way.

### Continuity projection for splines of odd degree

Suppose we are given $(Q_1^{(i)}, Q_2^{(i)})_{i=1}^I$, which are $(k + 1) \times (k + 1)$ matrices (not necessarily in $\Psi$), defining a piecewise polynomial as in equation 2 of the manuscript. Computing the projection $(X_*^{(i)}, Y_*^{(i)})_{i=1}^I$ of $(Q_1^{(i)}, Q_2^{(i)})_{i=1}^I$ onto $\mathcal{C}_1$ can be done by solving the following optimization problem:

$$(X_*^{(i)}, Y_*^{(i)})_{i=1}^I = \underset{(X^{(i)},Y^{(i)})_{i=1}^I}{\arg\min} \sum_{i=1}^I ||X^{(i)} - Q_1^{(i)}||_F^2 + ||Y^{(i)} - Q_2^{(i)}||_F^2$$
$$\text{s.t. } (t_i - t_{i-1})[t_i]^\top Y^{(i)}[t_i] = (t_{i+1} - t_i)[t_i]^\top X^{(i+1)}[t_i], \text{ for } i = 1, \ldots, I - 1$$

where $|| \cdot ||_F$ denotes the Frobenius norm and each constraint is merely forcing the piecewise function to be continuous at knot $i$ for $i = 1, \ldots, I - 1$. Note that this is a quadratic optimization problem

33rd Conference on Neural Information Processing Systems (NeurIPS 2019), Vancouver, Canada.

with linear constraints, and can be solved analytically. The corresponding Lagrangian is:

$$L((X^{(i)},Y^{(i)})_{i=1}^I,\lambda) = \sum_{i=1}^{I} ||X^{(i)}-Q_1^{(i)}||_F^2 + ||Y^{(i)}-Q_2^{(i)}||_F^2 + \sum_{i=1}^{I-1}\lambda_i\Big((t_i-t_{i-1})[t_i]^\top Y^{(i)}[t_i] - (t_{i+1}-t_i)[t_i]^\top X^{(i+1)}[t_i]\Big)$$

where $\lambda = (\lambda_1,\ldots,\lambda_{I-1})^\top \in \mathbb{R}^{I-1}$. By solving the KKT conditions, it can be verified that:

$$\begin{cases} X_*^{(i)} = Q_1^{(i)} + \frac{\lambda_{i-1}^*}{2}A_{i-1} \text{ , for } i=1,\ldots,I \\ Y_*^{(i)} = Q_2^{(i)} - \frac{c_i\lambda_i^*}{2}A_i \text{ , for } i=1,\ldots,I \\ \lambda_i^* = \frac{2}{1+c_i^2}\frac{[t_i]^\top(c_iQ_2^{(i)}-Q_1^{(i+1)})[t_i]}{([t_i]^\top[t_i])^2} \text{ , for } i=1,\ldots,I-1 \end{cases}$$

where $c_i = \frac{t_i-t_{i-1}}{t_{i+1}-t_i}$ for $i=1,\ldots,I-1$, $c_I=0$, $\lambda_0^*=0$, $\lambda_I^*=0$ and $A_i=[t_i][t_i]^\top$ for $i=0,\ldots,I$.

**Differentiability projection for splines of odd degree**

Analogously, computing the projection $(X_*^{(i)},Y_*^{(i)})_{i=1}^I$ of $(Q_1^{(i)},Q_2^{(i)})_{i=1}^I$ onto $\mathcal{C}_2$ can be done by solving the following optimization problem:

$$\begin{aligned}(X_*^{(i)},Y_*^{(i)})_{i=1}^I = \underset{(X^{(i)},Y^{(i)})_{i=1}^I}{\arg\min} & \sum_{i=1}^{I} ||X^{(i)}-Q_1^{(i)}||_F^2 + ||Y^{(i)}-Q_2^{(i)}||_F^2 \\ \text{s.t. } & -[t_i]^\top X^{(i)}[t_i] + [t_i]^\top Y^{(i)}[t_i] \\ & + (t_i-t_{i-1})[t_i']^\top Y^{(i)}[t_i] + (t_i-t_{i-1})[t_i]^\top Y^{(i)}[t_i'] \\ & = -[t_i]^\top X^{(i+1)}[t_i] + (t_{i+1}-t_i)[t_i']^\top X^{(i+1)}[t_i] \\ & + (t_{i+1}-t_i)[t_i]^\top X^{(i+1)}[t_i'] + [t_i]^\top Y^{(i+1)}[t_i], \text{ for } i=1,\ldots,I-1\end{aligned}$$

where $[t'] = (0,1,2t,3t^2,\ldots,kt^{k-1})^\top$ and each constraint is now forcing the values of the left and right derivatives of the piecewise function to match at knot $i$ for $i=1,\ldots,I-1$. Again, this is a quadratic optimization problem with linear constraints. By writing the Lagrangian and solving the KKT conditions, we get:

$$\begin{cases} X_*^{(i)} = Q_1^{(i)} + \frac{\lambda_i^*}{2}A_i - \frac{\lambda_{i-i}^*}{2}(A_{i-1}-(t_i-t_{i-1})M_{i-1}) \text{ , for } i=1,\ldots,I \\ Y_*^{(i)} = Q_2^{(i)} - \frac{\lambda_i^*}{2}(A_i+(t_i-t_{i-1})M_i) + \frac{\lambda_{i-1}^*}{2}A_{i-1} \text{ , for } i=1,\ldots,I \end{cases}$$

where $M_i = [t_i][t_i']^\top + [t_i'][t_i]^\top$ for $i=0,\ldots,I$ and:

$$\begin{aligned}&\lambda_{i-1}^*\Big([t_i]^\top(A_{i-1}-\frac{t_i-t_{i-1}}{2}M_{i-1})[t_i] + (t_i-t_{i-1})[t_i']^\top A_{i-1}[t_i]\Big) \\ &+ \lambda_i^*\Big([t_i]^\top(-2A_i - \frac{t_{i+1}-2t_i+t_{i-1}}{2}M_i)[t_i] \\ &\qquad + (t_{i+1}-2t_i+t_{i-1}-(t_i-t_{i-1})^2-(t_{i+1}-t_i)^2)[t_i']^\top M_i[t_i]\Big) \\ &+ \lambda_{i+1}^*\Big([t_i]^\top(A_{i+1}+\frac{t_{i+1}-t_i}{2}M_{i+1})[t_i] - (t_{i+1}-t_i)[t_i']^\top A_{i+1}[t_i]\Big) \\ &= [t_i]^\top(Q_1^{(i)}-Q_1^{(i+1)}-Q_2^{(i)}+Q_2^{(i+1)})[t_i] + 2[t_i']^\top((t_{i+1}-t_i)Q_1^{(i+1)}-(t_i-t_{i-1})Q_2^{(i)})[t_i]\end{aligned}$$

for $i=1,\ldots,I-1$ and again, $\lambda_0^*=0$ and $\lambda_I^*=0$. This is a tridiagonal system of $I-1$ linear equations with $I-1$ unknowns and can be solved efficiently in $O(I)$ time with simplified Gaussian elimination.

### Second differentiability projection for splines of odd degree

Finally, computing the projection $(X_*^{(i)}, Y_*^{(i)})_{i=1}^I$ of $(Q_1^{(i)}, Q_2^{(i)})_{i=1}^I$ onto $\mathcal{C}_2$ can be done by solving the following optimization problem:

$$
\begin{aligned}
(X_*^{(i)}, Y_*^{(i)})_{i=1}^I = \underset{(X^{(i)},Y^{(i)})_{i=1}^I}{\arg\min} & \sum_{i=1}^{I} ||X^{(i)} - Q_1^{(i)}||_F^2 + ||Y^{(i)} - Q_2^{(i)}||_F^2 \\
\text{s.t. } & -2[t_i']^\top X^{(i)}[t_i] - 2[t_i]^\top X^{(i)}[t_i'] + 2[t_i']^\top Y^{(i)}[t_i] + 2[t_i]^\top Y^{(i)}[t_i'] \\
& + (t_i - t_{i-1})[t_i'']^\top Y^{(i)}[t_i] + 2(t_i - t_{i-1})[t_i']^\top Y^{(i)}[t_i'] + (t_i - t_{i-1})[t_i]^\top Y^{(i)}[t_i''] \\
& = -2[t_i']^\top X^{(i+1)}[t_i] - 2[t_i]^\top X^{(i+1)}[t_i'] + (t_{i+1} - t_i)[t_i'']^\top X^{(i+1)}[t_i] \\
& + 2(t_{i+1} - t_i)[t_i']^\top X^{(i+1)}[t_i'] + (t_{i+1} - t_i)[t_i]^\top X^{(i+1)}[t_i''] + 2[t_i']^\top Y^{(i+1)}[t_i] \\
& + 2[t_i]^\top Y^{(i+1)}[t_i']
\end{aligned}
$$

where $[t''] = (0, 0, 2, 6t, \ldots, k(k-1)t^{k-2})^\top$ and each constraint is now forcing the values of the left and right second derivatives of the piecewise function to match at knot $i$ for $i = 1, \ldots, I-1$. Again, this is a quadratic optimization problem with linear constraints. By writing the Lagrangian and solving the KKT conditions, we get:

$$
\begin{cases}
X_*^{(i)} = Q_1^{(i)} + \lambda_i^* M_i - \frac{\lambda_{i-i}^*}{2} B_{i-1} \text{ , for } i = 1, \ldots, I \\
Y_*^{(i)} = Q_2^{(i)} - \frac{\lambda_i^*}{2} E_i + \lambda_{i-1}^* M_{i-1} \text{ , for } i = 1, \ldots, I
\end{cases}
$$

where $B_{i-1} = 2M_{i-1} - (t_i - t_{i-1})([t_{i-1}''][t_{i-1}]^\top + 2[t_{i-1}'][t_{i-1}']^\top + [t_{i-1}][t_{i-1}'']^\top)$ and $E_i = 2M_i - (t_i - t_{i-1})([t_i''][t_i]^\top + 2[t_i'][t_i']^\top + [t_i][t_i'']^\top)$ for $i = 1, \ldots, I$ and:

$$
\begin{aligned}
& \lambda_{i-1}^* \Big( [t_i']^\top (2B_{i-1} + 4M_{i-1})[t_i] + 2(t_i - t_{i-1})[t_i'']^\top M_{i-1}[t_i] + 2(t_i - t_{i-1})[t_i']^\top M_{i-1}[t_i'] \Big) \\
& + \lambda_i^* \Big( [t_i']^\top (-8M_i - 2E_i - 2B_i)[t_i] + [t_i'']^\top ((t_{i+1} - t_i)B_i - (t_i - t_{i-1})E_i)[t_i] \\
& \qquad + [t_i']^\top ((t_{i+1} - t_i)B_i - (t_i - t_{i-1})E_i)[t_i'] \Big) \\
& + \lambda_{i+1}^* \Big( [t_i']^\top (E_{i+1} + 4M_{i+1})[t_i] - 2(t_{i+1} - t_i)[t_i'']^\top M_{i+1}[t_i] - 2(t_{i+1} - t_i)[t_i']^\top M_{i+1}[t_i'] \Big) \\
& = 4[t_i']^\top (Q_1^{(i)} - Q_1^{(i+1)} - Q_2^{(i)} + Q_2^{(i+1)})[t_i] + 2[t_i'']^\top ((t_{i+1} - t_i)Q_1^{(i+1)} - (t_i - t_{i-1})Q_2^{(i)})[t_i] \\
& \quad + 2[t_i']^\top ((t_{i+1} - t_i)Q_1^{(i+1)} - (t_i - t_{i-1})Q_2^{(i)})[t_i'] \text{ , for } i = 1, \ldots, I-1
\end{aligned}
$$

where again, $\lambda_0^* = 0$ and $\lambda_I^* = 0$. Again, this is a tridiagonal system of $I-1$ linear equations with $I-1$ unknowns that can be solved efficiently.

## Appendix 3: Architectural choices and training parameters

For our simulated data experiment, the state of each LSTM has 100 units, and $\tilde{f}$ is a feed-forward neural network with ReLU activations and with 3 hidden layers, each one with 100 units. We apply 102 iterations of the method of alternating projections. For the feed-forward architecture in PfLDS, we also used 3 hidden layers, each with 100 units. We used a mini-batch of size 2 and the learning rate was 0.001. For the real data experiments we used the same choices, except the state of each LSTM has 25 units and $\tilde{f}$ is a feed-forward network with ReLU activations and with 3 hidden layers, each one with 10 units (we tried more complicated architectures but saw no improvement).

## Appendix 4: Data Preprocessing

### Reaching Data Preprocessing

We include only successful trials (i.e. when the primate reaches to the correct location) and use only spikes occurring in a window of $-100ms$ and $300ms$ from the time that movement starts. We also

reduce the total number of neurons as inference with our method requires one LSTM per neuron and having too many neurons renders training slow. In order to do so, we use the following GLM:

$$y_r \sim \text{Multinomial}\big(C, \text{softmax}(\tilde{K}_{r,\cdot}^\top \beta)\big)$$

where $y_r$ is the trial type of trial $r$, $C = 40$ is the number of trial types, $\tilde{K}_{r,\cdot} \in \mathbb{R}^N$ is a vector containing the (centered and standardized) number of spikes in trial $r$ for each of the $N = 223$ neurons, and $\beta \in \mathbb{R}^{N \times C}$ are the GLM parameters. We train the GLM using group lasso [40], where the groups are defined by neurons. That is, the GLM is trained through maximum likelihood with an added penalty:

$$\lambda \sum_{n=1}^{N} ||\beta_{n,\cdot}||_2^2$$

where $\beta_{n,\cdot}$ is the $n^{th}$ row of $\beta$. This makes it so that the coefficients in each group hit zero simultaneously. A neuron $n$ is removed if $||\hat{\beta}_{n,\cdot}|| = 0$. We use a regularization parameter $\lambda$ such that all but 20 neurons are removed. This provides a principled way of reducing the number of neurons while making sure that the kept neurons are useful. As PfLDS does not require the use of LSTMs, it can be run on the data without removing neurons. While doing this did increase performance of PfLDS, it did so very marginally and our model still heavily outperformed PfLDS.

**Cycling Data Preprocessing**

Once again, we only keep successful trials (i.e. when the primate pedals in the correct direction and speed) and reduce the total number of neurons $N = 256$ to 20 by using group lasso. Since each trial has a different length, we extend every trial to have the same length as the longest trial. We add no spikes to these extended time periods.
